# Supplementary material for: Dissonance Between Human and Machine Understanding
Source: arXiv:2101.07337 source file (2021-01-18)
Supplement: Supplementary file 1 [file appendix.tex]

\begin{figure}
    \includegraphics[width=0.4\textwidth]{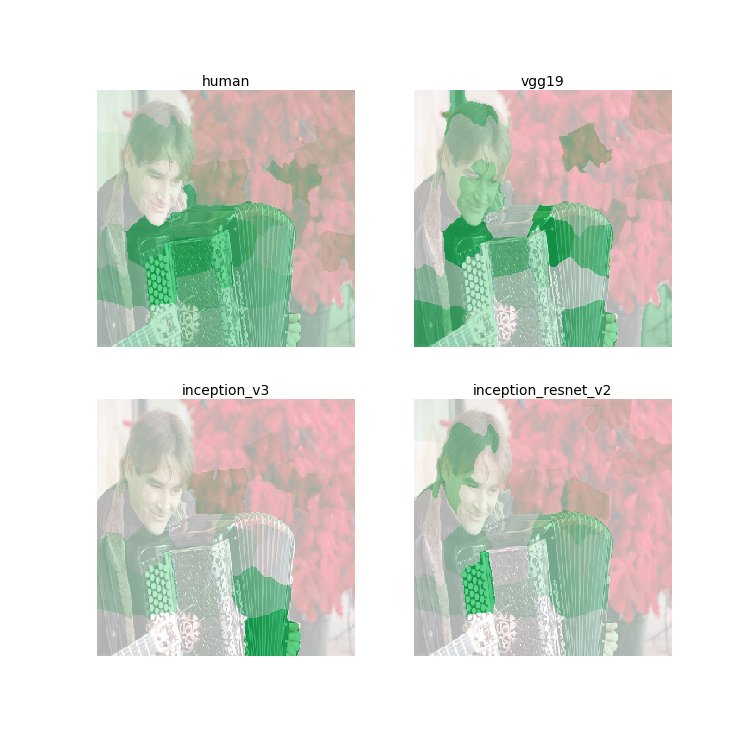}
    \caption{Heatmaps encoding order of segment importance for \texttt{accordion}}
    \label{fig:accordion}
\end{figure}

\begin{figure}
    \includegraphics[width=0.4\textwidth]{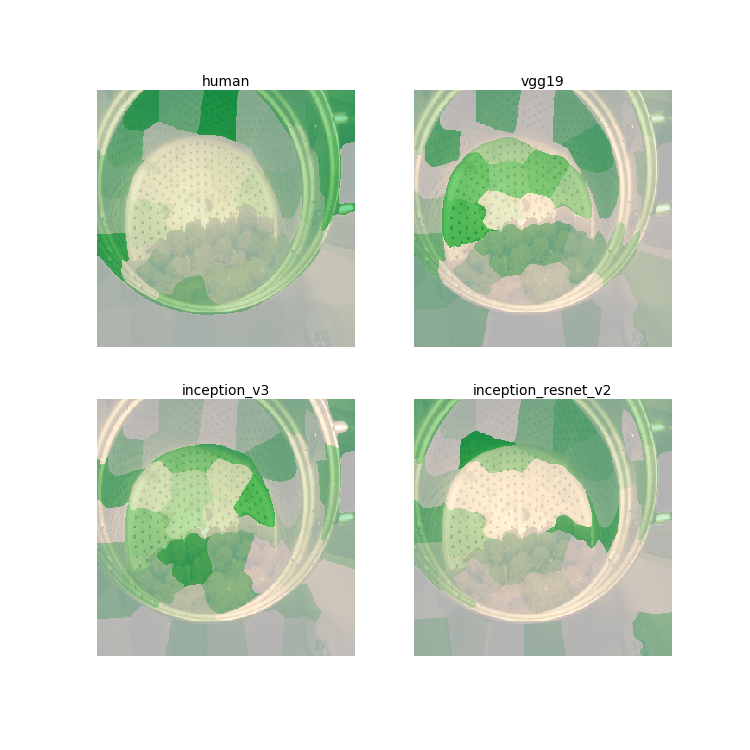}
    \caption{Heatmaps encoding order of segment importance for \texttt{strainer}}
    \label{fig:strainer}
\end{figure}

\begin{figure}
    \includegraphics[width=0.4\textwidth]{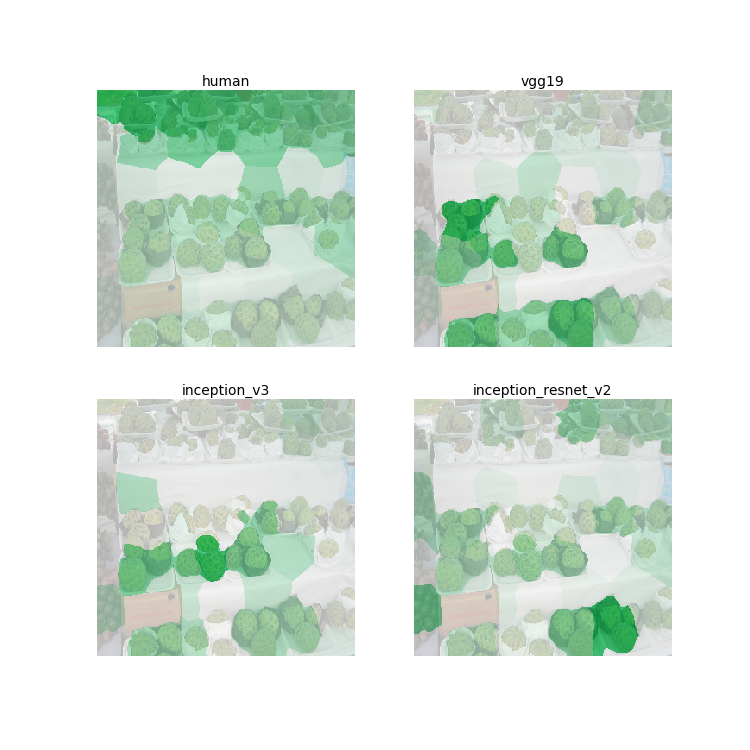}
    \caption{Heatmaps encoding order of segment importance for \texttt{custard apple}}
    \label{fig:capple}
\end{figure}

\begin{figure}
    \includegraphics[width=0.4\textwidth]{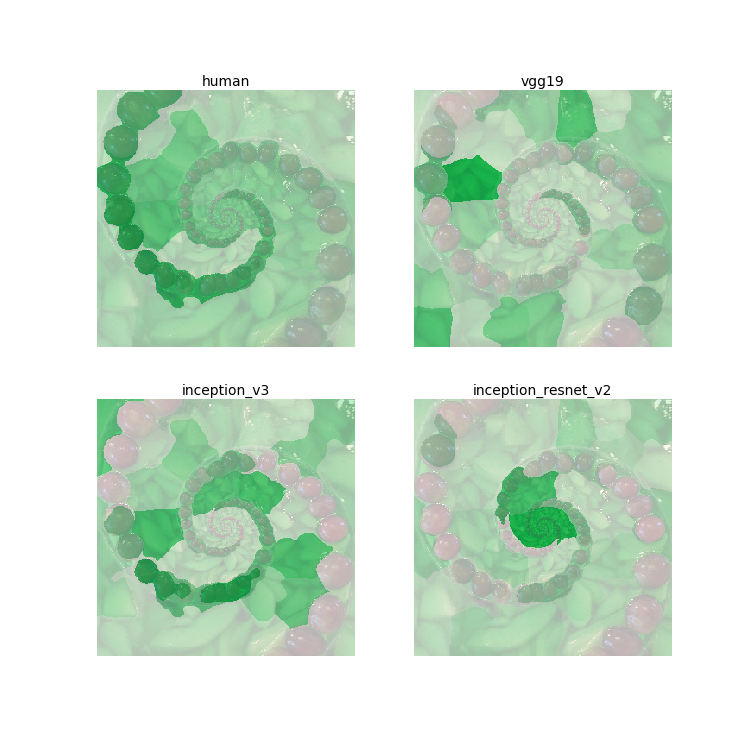}
    \caption{Heatmaps encoding order of segment importance for \texttt{coil}}
    \label{fig:coil}
\end{figure}
